# Supplementary material for: Unified description of high-energy nuclear collisions based on dynamical core--corona picture
Source: arXiv:2208.07029 source file (2022-08-15)
Supplement: Supplementary file 1 [file appendixA.tex]

\thispagestyle{fancy}

%--------------------------------------------------------
\section{Quantum Chromo Dynamics (QCD)}
Quantum Chromo Dynamics (QCD) is a fundamental theory to describe strong force.

There are two notable characteristics which are "confinement of color" and "asymptotic freedom".

\subsection{Color confinement}
It is said to be that quarks cannot be extracted as one unit, since they are confined to form color singlet.

\subsection{Asymptotic freedom}
Asymptotic freedom of quarks was proposed by Wilchek and Gross.

%--------------------------------------------------------

\subsection{Sigma model}
%================

Then one can rewrite the QCD Lagrangian density as follows, 

\vspace{10mm}

By expressing the mass term with a combined field of isoscalar $\sigma$ and isovector $\vec{\pi}$, one can get a form of Lagrangian in a chiral-symmetry form.

The potential term, for the case that $\nu^2>0$, becomes a wine-bottle shape sitting on $\sigma$-$\vec{\pi}$ plane. Thus, the origin is no longer a lowest energy state, but the $\sigma^2+\vec{\pi}^2=\nu^2$ is. Now one can choose a particular vacuum from this edge of the wine bottle. By choosing a vacuum at $\sigma=\nu$ and $\vec{\nu}=0$ and shifting the Lagrangian with  $\sigma\rightarrow\sigma+\nu$ and $\vec{\pi}\rightarrow\vec{\pi}$, one can get the following form. 
This Lagrangian is now not invariant under axial transformation, which means, chiral symmetry is spontaneously broken.
The important thing to notice here is that a mass term of $\vec{\pi}$ does not appear while that of $\sigma$ does. From this consequence, it is said that the isovector $\vec{\pi}$ is a Nambu-Goldstone boson, mass-less boson which appears due to the spontaneous chiral symmetry breaking.

%==============================
