# Supplementary material for: Unified description of high-energy nuclear collisions based on dynamical core--corona picture
Source: arXiv:2208.07029 source file (2022-08-15)
Supplement: Supplementary file 2 [file appendixB.tex]

\thispagestyle{fancy}
Milne coordinate is adopted in hydrodynamic simulations. Since Milne coordinate is so called a curved space, it is convenient to have some knowledge on general relativity.

\section{Basics}

\subsection{Metric and transformation matrix}

\begin{align}
    ds^2 = \eta_{\mu\nu} dx^{\mu} dx^{\nu}, 
\end{align}
\begin{align}
    \eta_{\mu\nu} =
    \begin{pmatrix}
      1 & 0 & 0 & 0 \\
      0 & -1 & 0 & 0 \\ 
      0 & 0 & -1 & 0 \\ 
      0 & 0 & 0 & -1 
    \end{pmatrix}
\end{align}

\begin{align}
    ds^2 = g_{\alpha\beta} d\tilde{x}^{\alpha} d\tilde{x}^{\beta}, 
\end{align}
\begin{align}
     g_{\alpha\beta} =  \frac{\partial x^{\mu}}{\partial\tilde{x}^{\alpha} }\frac{\partial x^\nu}{\partial\tilde{x}^{\beta}} \eta_{\mu\nu}, 
\end{align}

\begin{align}
    d\bm{x} = dx^\mu \bm{e}_\mu = d\tilde{x}^\alpha \tilde{\bm{e}}_\alpha
\end{align}

\begin{align}
    \bm{e}_\mu = \epsilon^\alpha_\mu \tilde{\bm{e}}_\alpha
\end{align}
\begin{align}
    d\tilde{x}^\alpha = \epsilon^\alpha_\mu dx^\mu 
\end{align}

\begin{align}
    \epsilon^\alpha_{\mu} = \frac{\partial\tilde{x}^\alpha}{\partial x^\mu}
\end{align}

\begin{align}
    ds^2 = (dx^\mu \bm{e}_\mu) \cdot (dx^\nu \bm{e}_\nu)  = dx^\mu dx^\nu g_{\mu\nu}
\end{align}

\begin{align}
    g_{\mu\nu} = \bm{e}_{\mu} \cdot \bm{e}_\nu
\end{align}

\subsection{Christoffel symbol}

\begin{align}
    \Gamma^\alpha_{\mu\beta} = \frac{\partial \tilde{x}^\alpha}{\partial x^\nu} \frac{\partial^2 x^\nu}{\partial x^\mu \partial \tilde{x}^\beta}
\end{align}

\begin{align}
    \Gamma = \Gamma_{\beta \gamma \alpha } g^{\delta \alpha} = \frac{1}{2} g^{\gamma \alpha} (g_{\gamma \beta, \delta} - g_{\delta \gamma , \beta}+g_{\beta \gamma , \delta}) 
\end{align}
\begin{align}
    A^\mu_{;\mu} &= A^{\mu}_{,\mu} + \Gamma^{\mu}_{\mu\xi} A^\xi \nonumber \\
& = \frac{1}{\sqrt{-g}} \frac{\partial}{\partial x^\mu} (\sqrt{-g}A^\mu)
\end{align}
Note that
\begin{align}
    \det |\eta_{\mu\nu}| &= \det \left|\frac{\partial x^\mu}{\partial \tilde{x}^\alpha} \frac{\partial x^\nu}{\partial \tilde{x}^\beta} g_{\alpha \beta} \right| \nonumber \\
 \Leftrightarrow   -1 &= \det \left| \frac{\partial x}{\partial \tilde{x}}\right|^2 \det |g| \nonumber \\\
 \Leftrightarrow &  \det |g| \equiv g <0
\end{align}

\begin{align}
    B^{\mu\nu}_{;\mu} = \frac{1}{\sqrt{-g}}\partial_\mu (\sqrt{-g}B^{\mu\nu}) + \Gamma_{\xi\mu}^\nu B^{\mu\xi}
\end{align}

\section{Milne and Cartesian}
