# Supplementary material for: Unified description of high-energy nuclear collisions based on dynamical core--corona picture
Source: arXiv:2208.07029 source file (2022-08-15)
Supplement: Supplementary file 3 [file appendixC.tex]

\thispagestyle{fancy}
%In the last section, we get the relativistic hydrodynamic equations in a convenient form for numerical calculation.
As I explained in Sec.~\ref{sebsec:DYNAMICAL_INITIALIZATION} of chapter 2, relativistic hydrodynamics is used to describe the space-time evolution of the QGP.
In this Appendix, I would like to access the details of the numerical treatment of hydrodynamic equations.

The code of (3+1)-D hydrodynamics used in this thesis is built by Tachibana in Ref.~\cite{Tachibana:2014yai}.

In this code, the (3+1)-D hydrodynamics is solved with the {\it{Peacewise Parabolic Method}} (PPM).
The PPM is a robust algorithm to solve the Riemann problem with shock waves. 
The first implementation to numerical simulations of relativistic heavy-ion collisions was done by Hirano in Ref.~\cite{Hirano:2000eu}.

Now we need to know how to solve them numerically in a discretized-cell space.  
The problem one has to handle is the space-time evolution of a distribution of the density $U$ as shown in Fig.
Since we discretize space into cells in numerical simulation of hydrodynamics, $U$ is assumed to be constant in each cell. 
Thus, there is a discontinuity of $U$ between two adjacent cells. 
The initial value problem with such a discontinuity in numerical simulation of hydrodynamics is called, Riemann problem. 

\section{PPM}
The numerical method for solving hydrodynamics is a huge topic as itself. Especially, one has to be careful in treatment of compressible fluids because shock wave can arise in a simulation, and which can make a simulation numerically unstable. 

The Peacewise Parabolic Method (PPM) is a robust algorithm to solve the Riemann problem with shock waves. The PPM was employed to numerical simulations of relativistic heavy-ion collisions at first time in Ref.~\cite{Hirano:2000eu}.
This work uses the PPM in (3+1)-D hydrodynamic simulations.

\subsection{Interpolation function, $U(x)$}
As a first step of the PPM, one starts with interpolating density of each cell so that one can analytically obtain solutions of Riemann problem. 
Suppose that the $j$th cell has density $U_j$, where $j$ is a cell index.
The $j$th cell is defined to be located within $x_{j-\frac{1}{2}}< x < x_{j+\frac{1}{2}}$ with a cell width $\Delta x = x_{j+\frac{1}{2}} - x_{j-\frac{1}{2}}$.
Here, we replace the $U_j$ with a smooth interpolation function $U_j(x)$ defined as,
\begin{align}
    \label{eq:interpolated_func}
    \dis U_{j} = \int_{x_{j-\frac{1}{2}}}^{x_{j+\frac{1}{2}}} U_j(x) dx.
\end{align}
In the PPM, interpolation function is given as a hyperbolic form.
If we replace variable as $X=\frac{x-x_{j-\frac{1}{2}}}{\Delta x}$,  the interpolation function $U_j(x)$ can be expressed as,
\begin{align}
    \label{eq:interpolation_func}
        U_j(X) = aX^2 + bX + c,
\end{align}
where $a, b,$ and $c$ are unknown constants.
The boundary conditions of $U_j(X)$ given as $U_j(X=0) = U_{j,L}$ and $U_j(X=1) = U_{j,R}$ and integration of Eq.~\refbra{eq:interpolation_func} from $X=0$ to $X=1$ gives simultaneous equations. Solving the equations, one can obtain
\begin{align}
    a &= -6\left[  U_j - \frac{1}{2} \left( U_{j,R} + U_{j,L} \right)\right] \equiv U_{j,6}, \\
    b &= U_{j,6} + (U_{j,R}-U_{j,L}) \equiv U_{j,6} + \Delta U_j, \\
    c&= U_{j,L}.
\end{align}
Then finally the interpolation function $U_{j}(x)$ becomes,
\begin{align}
    \label{eq:INTERPOLATION_Ux}
    U_j(x) = - U_{j,6} \left(\frac{x-x_{j-\frac{1}{2}}}{\Delta x}\right)^2  + (U_{j,6} + \Delta U_{j} ) \frac{x-x_{j-\frac{1}{2}}}{\Delta x} + U_{j, L}.
\end{align}

\subsection{Density at edge of cell, $U_{j,R}$ and $U_{j,L}$}
The next problem is how we obtain the $U_{j, R}$ and $U_{j, L}$ as a function of density $U$ which is known value.  
Here we analytically obtain each value of the $U_{j, R}$ and $U_{j, L}$ from 4-adjacent cells.
Suppose that there is the distribution of density $U$ shown in Fig. The cells are labeled as $j-1, j, j+1$ and $j+2$ respectively. First we assume that the integral of $U(x)$ can be parametrized as a quartic function,
\begin{align}
    \label{eq:interpolation_fourcells}
    \mathcal{U}(x) &= \int_{x_{j-\frac{3}{2}}}^x d\xi U(\xi)   \\
    \label{eq:interpolation_fourcells_ana}
     & = ax^4 + bx^3 + cx^2 + dx + e,
\end{align}
where $a,b,c,d$ and $e$ are unknown constants. Note that Eq.~\refbra{eq:interpolation_fourcells} is defined within $x_{j-\frac{3}{2}} < x < x_{j+\frac{5}{2}}$ so the integrated interpolation function $U(\xi)$ is assumed to be defined globally within this region. Then values at cell boundaries can be calculated as,
\begin{align}
\label{eq:boundary_value}
U_{j,R} = U(x_{j+\frac{1}{2}})  = \left. \frac{d\mathcal{U}}{dx}\right|_{x=x_{j+\frac{1}{2}}}.
\end{align}
The quartic function is employed because we want to obtain $U_{j, R}$ and $U_{j, L}$ from $U$ of 4-adjacent cells.
One can solve above equations by assuming $x_{j+\frac{1}{2}}=0$ and $\mathrm{U}(x_{j-\frac{3}{2}})=0$ without loss of generality.

Since we know $U$ at each cell, integral of Eq.~\refbra{eq:interpolation_fourcells} is easily obtained by taking sum of products of each $U$ and $\Delta x$. One would obtain the following equations:
\begin{align}
\label{eq:coupledeqA}
\mathcal{U}(x_{j-\frac{3}{2}}) &= \int_{x_{j-\frac{3}{2}}}^{x_{j-\frac{1}{2}}} d\xi U(\xi) = 0, \\
\label{eq:coupledeqB}
\mathcal{U}(x_{j-\frac{1}{2}}) &=
\int_{x_{j-\frac{3}{2}}}^{x_{j-\frac{1}{2}}} d\xi U(\xi) = U_{j-1}\Delta x, \\
\label{eq:coupledeqC}
\mathcal{U}(x_{j+\frac{1}{2}}) &=
\int_{x_{j-\frac{3}{2}}}^{x_{j+\frac{1}{2}}} d\xi U(\xi) = (U_{j-1}+U_{j})\Delta x, \\
\label{eq:coupledeqD}
\mathcal{U}(x_{j+\frac{3}{2}}) &=
\int_{x_{j-\frac{3}{2}}}^{x_{j+\frac{3}{2}}} d\xi U(\xi) = (U_{j-1}+U_{j}+U_{j+1})\Delta x,  \\
\label{eq:coupledeqE}
\mathcal{U}(x_{j+\frac{5}{2}}) &=
\int_{x_{j-\frac{3}{2}}}^{x_{j+\frac{5}{2}}} d\xi U(\xi) = (U_{j-1}+U_{j}+U_{j+1}+U_{j+2})\Delta x.
\end{align}

On the other hand, by inserting $x_{j- \frac{3}{2}}=-2\Delta x$, $x_{j-\frac{1}{2}}=-\Delta x$, $x_{j+\frac{1}{2}}=0$,  $x_{j+ \frac{3}{2}}=\Delta x$, , and $x_{j+\frac{5}{2}}=2\Delta x$ into Eq.~\refbra{eq:interpolation_fourcells_ana}, one obtain,
\begin{align}
\label{eq:coupled_eqA}
\mathcal{U}(-2\Delta x) &= 16a \Delta x ^4 - 8b\Delta x^3 + 4c\Delta x^2 -2 d\Delta x + e, \\
\label{eq:coupled_eqB}
\mathcal{U}(-\Delta x) &=
a\Delta x^4 - b \Delta x^3 + c\Dx^2 - d \Dx + e,  \\
\label{eq:coupled_eqC}
\mathcal{U}(0) &= e, \\
\label{eq:coupled_eqD}
\mathcal{U}(\Dx) &=
a \Dx^4 + b\Dx^3 + c\Dx^2 + e\Dx,  \\
\label{eq:coupled_eqE}
\mathcal{U}(2\Delta x) &=
16 a \Dx^4 + 8b \Dx^3 + 4c \Dx^2 + 2d \Dx + e.
\end{align}

Then, Eq.~\refbra{eq:coupled_eqA} to \refbra{eq:coupled_eqE} and Eq.~\refbra{eq:coupledeqA} to \refbra{eq:coupledeqE} lead to 5 simultaneous equations which determine 5 unknown constants in Eq.~\refbra{eq:interpolation_fourcells_ana}.

Finally, $a, b, c, d$, and $e$ are obtained as,
\begin{align}
    a &= (-U_{j-1} + 3U_j -3U_{j+1} +U_{j+2})/24\Dx^3, \\
    b &= -(-U_{j-1} + U_j +U_{j+1} -U_{j+2})/12\Dx^2, \\
    c &= -(-U_{j-1} + 15U_j -15U_{j+1} +U_{j+2})/40\Dx, \\
    d &= (U_j + U_{j+1})/2 + (-U_{j-1} + U_j +U_{j+1} -U_{j+2})/12, \\
    e&= (U_{j-1} + U_{j}) \Dx.
\end{align}

Finally, $U_{j, R}$ becomes,
\begin{align}
    \label{eq:UR}
    U_{j,R} &= U(x_{j+\frac{1}{2}}) \nonumber \\
    &= d \nonumber \\
    &=\frac{U_j+U_{j+1}}{2} + \frac{(U_{j+1} - U_{j-1}) - (U_{j+2} - U_{j})}{12}  \nonumber \\
    & = \frac{7}{12} (U_{j}+ U_{j+1}) -\frac{1}{12} (U_{j+2} + U_{j-1}).
\end{align}

On the other hand, $U_{j,L}$ becomes,
\begin{align}
    \label{eq:UL}
    U_{j,L} &= U(x_{j-\frac{1}{2}}) \nonumber \\
    & = \frac{7}{12} (U_{j-1}+ U_{j}) -\frac{1}{12} (U_{j+1} + U_{j-2}).
\end{align}

\subsection{Monotonicity of $U_R$ and $U_L$}
There are some cases where monotonicity of $U_R$ and $U_L$ is lost in $x_{j-\frac{1}{2}}<x<x_{j+\frac{1}{2}}$, and which we need to fix.
(a) First case is when $U_j$, density of the $i$th cell, does not take the value between $U_{j,R}$ and $U_{j,L}$.
(b) Second case is when $U_j$ is in between $U_{j, R}$ and $U_{j,L}$ but the interpolation function $U_j(x)$ has minimum or maximum value in $x_{j-\frac{1}{2}}<x<x_{j+\frac{1}{2}}$.

To impose monotonicity on the interpolation function, we replace the values of $U_{j,L}$ and $U_{j,R}$ as follows.
\begin{align}
\label{eq:Mono_a}
    U_{R,j} \rightarrow U_{j}, \ U_{L, j} \rightarrow U_{j} \nonumber \\ 
    \mathrm{if} \  (U_{R,j}-U_{j})(U_{L,j}-U_{j})\leq0,
\end{align}
\begin{align}
\label{eq:Mono_bm}
    U_{j,L} \rightarrow 3U_{j}-2U_{R,j} \nonumber \\
    \mathrm{if} \ \Delta U_{j}U_{j,6} > \Delta U_{j}^2,
\end{align}
\begin{align}
\label{eq:Mono_bp}
    U_{j,R} \rightarrow 3U_{j}-2U_{L,j} \nonumber \\
    \mathrm{if} \ \Delta U_{j}U_{j,6} < -\Delta U_{j}^2.
\end{align}
The condition in Eq.~\refbra{eq:Mono_a} corresponds to the case of (a) while ones in Eq.~\refbra{eq:Mono_bm} and \refbra{eq:Mono_bp} correspond to the case of (b). Each situation is shown in Fig.().
For the case of (a), $U_{R,j}$ and $U_{L,j}$ are replaced so that the interpolation function becomes constant within $x_{j-\frac{1}{2}}<x<x_{j+\frac{1}{2}}$.
On the other hand, for the case of (b), $U_{R,j}$ or $U_{L,j}$ is replaced so that the interpolation function takes its maximum or minimum at the edge of the $j$th cell keeping the value of $U_j$. If $U_{R,j}$ is closer to the maximum or minimum point $U_{L,j}$ is moved while $U_{R,j}$ and $U_{j}$ is fixed, and vice versa.

Just in case, note that the conditions in Eq.~\refbra{eq:Mono_bm} and \refbra{eq:Mono_bp} are obtained as follows.
Remember that the interpolation function is expressed as Eq.~\refbra{eq:INTERPOLATION_Ux}. By replacing $\frac{x-x_{j-\frac{1}{2}}}{\Dx}$ with $X$ and taking derivative with $X$, one would obtain
\begin{align}
    \frac{dU_j(X)}{dX} = -2U_{6,j}X+U_{6,j}+\Delta U_j, \ (0\leq X\leq 1).
\end{align}
This leads to the following conditions of non-monotonicity,
\begin{align}
    & 0\leq\frac{U_{6,j}+\Delta U_j}{2U_{6,j}}\leq 1 \nonumber \\
    \Leftrightarrow \  & -U_{6,j}\leq\Delta U_j \leq U_{6,j} \nonumber \\
    \Leftrightarrow \  & |\Delta U_j |>| U_{6,j}|.
\end{align}
The conditions in Eq.~\refbra{eq:Mono_bm} and Eq.~\refbra{eq:Mono_bp} corresponds to the cases where $\Delta U_j<0$ and $0<\Delta U_j$, respectively.

\subsection{Contribution of propagating $U_R$ and $U_L$ in $\Delta t$}
Now we have the interpolation function of Eq.~\refbra{eq:INTERPOLATION_Ux} as a function of density $U$ of each cell at a fixed time. 
However, in the form of Eq.~\refbra{eq:UR} and \refbra{eq:UL}, there
How fluids propagate can be evaluated by using a signal velocity. During $\Delta t$, discontinuity flows from the right and left into the constant region, as shown in Fig.().
Average values of interpolation functions $U(x)$ that flow into the boundary is obtained as follows.
\begin{align}
\label{eq:ave_UL}
    \bar{U}_{j+1,L}& = \frac{1}{|b_{j+\frac{1}{2},r}|\Delta t} \int_{x_{j+\frac{1}{2}}}^{x_{j+\frac{1}{2}} + |b_{j+\frac{1}{2}, r}|\Delta t} U_{j+1} (x) dx, \\
\label{eq:ave_UR}
    \bar{U}_{j,R} &= \frac{1}{|b_{j,l}|\Delta t} \int^{x_{j+\frac{1}{2}}}_{x_{j+\frac{1}{2}} - |b_{j+\frac{1}{2}, r}|\Delta t} U_{j} (x) dx 
\end{align}

\begin{align}
    b = \frac{v+c}{1+vc}
\end{align}

The Eq.~\refbra{eq:ave_UL} becomes,
\begin{align}
    \bar{U}_{L, j+1} &= \frac{1}{|b|\Delta t } \int_{x_{j+\frac{1}{2}}}^{x_{j+\frac{1}{2}} + |b|\Delta t} dx U_{j+1} (x) \nonumber \\
    & = \frac{1}{|b|\Delta t} \int_{x_{j+\frac{1}{2}}}^{x_{j+\frac{1}{2}} + |b|\Delta t} dx U_{L, j+1} + \frac{x-x_{j+\frac{1}{2}}}{\Dx}\left[ \Delta U_{j+1} + U_{6, j+1} \left(1-\frac{x-x_{j+\frac{1}{2}} }{\Dx}\right) \right] \nonumber \\
    & = U_{L, j+1} + \frac{1}{|b|\Delta t} \left[ 
    \int_{x_{j+\frac{1}{2}}}^{x_{j+\frac{1}{2}} + |b|\Delta t} dx \frac{x-x_{j+\frac{1}{2}}}{\Dx} \Delta U_{j+1} \right. \nonumber \\ 
     & \hspace{30mm} \left. + \int_{x_{j+\frac{1}{2}}}^{x_{j+\frac{1}{2}} + |b|\Delta t} dx \left[ \frac{x-x_{j+\frac{1}{2}}}{\Delta x} U_{6, j+1} - \left( \frac{x-x_{j+\frac{1}{2}}}{\Dx}\right)^2 U_{6, j+1} \right] \right] \nonumber.
\end{align}
The first term in the integral can be computed as,
\begin{align}
    \int_{x_{j+\frac{1}{2}}}^{x_{j+\frac{1}{2}} + |b|\Delta t} dx  \frac{x-x_{j+\frac{1}{2}}}{\Dx} \Delta U_{j+1} 
    &= \int_{x_{j+\frac{1}{2}}}^{x_{j+\frac{1}{2}} + |b|\Delta t} dx \frac{\Delta U}{\Delta x} - \int_{x_{j+\frac{1}{2}}}^{x_{j+\frac{1}{2}} + |b|\Delta t} dx \frac{\Delta U}{\Dx} x_{j+\frac{1}{2}} \nonumber\\
    & = \left[ \frac{1}{2} \left[(x_{j+\frac{1}{2}} + |b|\Delta t)^2 - x_{j+\frac{1}{2}}^2 \right] - (|b|\Delta t x_{j+\frac{1}{2}}) \right] \frac{\Delta U}{\Dx} \nonumber \\
    & = \frac{1}{2} |b|^2 \Delta t^2 \frac{\Delta U}{\Delta x}
\end{align}

The second term becomes,
\begin{align}
    \dis & \int_{x_{j+\frac{1}{2}}}^{x_{j+\frac{1}{2}} + |b|\Delta t} dx \left[ \frac{x-x_{j+\frac{1}{2}}}{\Delta x} U_{6, j+1} - \left( \frac{x-x_{j+\frac{1}{2}}}{\Dx}\right)^2 U_{6, j+1} \right] \nonumber \\
    &= \frac{U_6}{|b|\Delta t} \left[\frac{1}{2\Dx} |b|^2 \Delta t^2  \right] - \frac{U_6}{|b|\Delta t \Dx^2} \left[\frac{1}{3} |b|^3 \Delta t^3\right] \nonumber \\
    & = \frac{U_6}{2\Dx}|b|\Delta t \left[ 1- \frac{2|b|\Delta t}{3\Dx}\right].
\end{align}

Finally, one would obtain
\begin{align}
    \bar{U}_{L,j+1}=U_{L,j+1} + \frac{b\Delta t }{2\Dx} \left[\Delta U + \left(1-\frac{2b\Delta t}{3\Dx}U_{6} \right)\right].
\end{align}

In the same way, \refbra{eq:UR} is expressed as 
\begin{align}
    \bar{U}_R = U_R - \frac{b\Delta t }{2\Dx} \left[\Delta U - \left( 1 - \frac{2b\Delta t}{3\Delta x}U_6 \right)\right].
\end{align}
