# Supplementary material for: Unified description of high-energy nuclear collisions based on dynamical core--corona picture
Source: arXiv:2208.07029 source file (2022-08-15)
Supplement: Supplementary file 4 [file appendixD.tex]

\thispagestyle{fancy}

%--------------------------------------------------------
\section{Statistics}

\subsection{Standard errors}
When it comes to deal with event-by-event fluctuating data, it must be inevitable to get familiar with statistical analysis. 

Although it would be quite straight-forward to get average and error-bar if you have simple event-by-event data set, that is not always the case.
For instance, if one uses Monte-Carlo event generator it is sometimes necessary to generate {\it{weighted}} events to reduce statistical errors. Suppose that one needs to analyze centrality dependence of certain observable. However, because a cross-section of colliding nuclei is proportional to an impact parameter, i.e., $d\sigma(b)/db \propto b$, it would be hard to gain statistics of collisions with small impact-parameter. One feasible way to solve this issue is to generate weighted events by sampling impact parameter according to some probability distributions, for instance, Gaussian function centered at zero. An inverse of the factor of Gaussian function corresponds to a weight of the event. This enables us to obtain enough statistics of collisions with small impact parameters.
On the other hand, in order to get event-average, one needs to take into account of the weights in statistical analysis.

In this section, I summarize how to calculate standard errors in weighted events. Definitions of standard errors for two different weighting methods are explained below. First, error bars in weighted events where each event is able to be counted as one complete event. Second, those where each event is $\it{not}$ able to be counted as one complete event.

Before going to a discussion of weighted event, I define average $\bar{x}$, unbiased sample variance $\sigma^2$ (here after I call this variance for simplicity), and corresponding standard error $\mathrm{SE}$ in un-weighted events.

\begin{equation}
\begin{aligned}
\label{eq:statval_unweighted}
    \bar{x} &=& \frac{\dis\sum_i^\Nev x_i}{\dis\sum_j^\Nev 1}, \hspace{5mm}
    \sigma^2 &=& \frac{\dis\sum_i^\Nev (x_i - \bar{x})^2}{\dis\sum_j^\Nev 1}, \hspace{5mm}
    \mathrm{SE} &=& \sqrt{\frac{\sigma^2}{\Nev}},
\end{aligned}
\end{equation}

\noindent 
where $x_i$ is a observable from a $i$th event and $\Nev$ is the number of event that one wants to analyze.
It is often the case with that there is not so much problem if one uses unbiased sample variance instead of biased one as an error bar in plots, since we often perform a number of event such as $\Nev >> 1$.

If the events are weighted and each produced event is able to be counted as one complete event, each definition in Eq.~\refbra{eq:statval_unweighted} becomes as follows.

\begin{equation}
\begin{aligned}
\label{eq:statval_weighted_normal}
    \bar{x} &=& \frac{\dis\sum_i^\Nev x_i w_i}{\dis\sum_j^\Nev w_j}, \hspace{5mm}
    \sigma^2 &=& \frac{\dis\sum_i^\Nev w_i (x_i - \bar{x})^2}{\dis\sum_j^\Nev w_j}, \hspace{5mm}
    \mathrm{SE} &=& \sqrt{\frac{\sigma^2}{\Nev}},
\end{aligned}
\end{equation}
\noindent
where $w_i$ is a weight of the $i$th event. For the variance, it is convenient to write down the value only with event-by-event variables to avoid adding an extra for-loop obtaining average in an analysis code.
Inserting the definition of average $\bar{x}$, one can readily obtain 
\begin{align}
    \sigma^2 = \frac{\dis\sum_i^\Nev w_i x_i^2 \sum_k^\Nev w_k 
                          -  \LSq \sum_i^\Nev x_iw_i \RSq^2} 
    { \dis \LSq \sum_j^\Nev w_j  \RSq^2}.
\end{align}

Next I discuss the case if one generated event is not able to be counted as one complete event.
In this case, we have to re-define each value since definition of ``event-average'' is different from the above one.

To make a discussion clear, let us think about one specific example.
When we try to get event-average of $\pT$ spectra using event-generator, it is often the case that it is hard to get enough statistics of events with high $\pT$ particle productions since a cross-section of such a high $\pT$ event is small.
To resolve this difficulty, one can specify transverse momentum produced in a hard process such as 2$\rightarrow$2, which is often denoted as $\hat{p}_T$, to generate high $\pT$ events. However, in order to get event-average of $\pT$ spectra, since a cross-section of such an event should be smaller than a total cross-section, a weight must be assigned to each data set generated with a certain range of $\hat{p}_T$. A weight is a fraction of an average of cross-sections of a certain range of $\hat{p}_T$ event to a total cross-section, $w_i = \sigma_{i}/\sigma_{\mathrm{tot}}$ \footnote{Ideally speaking, standard errors for the average of cross-section should be considered. In this discussion I just neglect them for simplicity.}.
Suppose that one generates $N_\pThat$ event for $n$ each range of $\pThat$, and the number of total generated event is $\Nev$, i.e., $\Nev = \sum_i^n N_\pThat = n N_\pThat$. Note that the weight is normalized as $\sum_i^n w_i = \sum_i^n \sigma_i/\sigma_{\mathrm{tot}} = 1$. 
In this case, to get straight to the point, each value in Eq.~\refbra{eq:statval_unweighted} becomes 

\begin{equation}
    \begin{aligned}
    \label{eq:statval_weighted}
            \bar{x} &=& \frac{\dis\sum_i^\Nev x_i w_i}{\dis\sum_j^\Nev w_j}, \hspace{5mm}
            \sigma^2 &=& \frac{\dis \sum_i^\Nev  \LSq x_i w_i \RSq^2}{\dis\sum_j^\Nev w_j} - \LSq \frac{\dis \sum_i^\Nev x_i w_i}{\dis \sum_j^\Nev w_j} \RSq^2, \hspace{5mm}
            \mathrm{SE} &=& \sqrt{\frac{\sigma^2}{\dis \sum_i^\Nev w_i}}.
    \end{aligned}
\end{equation}

\noindent
These can be understood when one back to the definition of event-average.
In the above case, one event is composed of each range of $\pThat$ and each data set of $\pThat$ has a corresponding weight.
This means that an observable value of one complete event corresponds to $x_i^\prime \defeq \sum_j^n x_{ij} w_j$ where $x_{ij}$ is a observable value of the $i$th event generated with the $j$th range of $\pThat$. This $x_i^\prime$ is related to $x_i$ in Eq.~\refbra{eq:statval_weighted} as

\begin{align}
    \dis \sum_i^\Nev x_i w_i = \sum_i^{N_\pThat}\sum_j^n x_{ij} w_j =  \sum_i^{N_\pThat} x_i^\prime.
\end{align}

\noindent
It would get clear if one rewrite Eq.~\refbra{eq:statval_weighted} with these definition.
Remembering that $\sum_i^\Nev w_i = N_\pThat$, average, variance and standard error become 

\begin{align}
\label{eq:average_weighted_clear}
    \bar{x} = \frac{\dis \sum_i^{N_{\pThat}} x_i^\prime}{N_\pThat},
\end{align}

\begin{equation}
    \begin{aligned}
    \label{eq:variance_weighted_clear}
            \sigma^2 &=& \frac{\dis \sum_i^{N_{\pThat}} \sum_j^{n}  \LSq x_{ij} w_i \RSq^2}{N_\pThat}  
            - \LSq \frac{ \sum_i^{N_\pThat} x_i^\prime }{N_\pThat} \RSq^2 \\
                    &\approx& \frac{\dis \sum_i^{N_{\pThat}} {x_i^\prime}^2 }{N_\pThat}  
            - \LSq \frac{ \sum_i^{N_\pThat} x_i^\prime }{N_\pThat} \RSq^2,
    \end{aligned}
\end{equation}

\begin{align}
\label{eq:SE_weighted_clear}
                \mathrm{SE} = \sqrt{\frac{\sigma^2}{N_\pThat}}.
\end{align}

From first to second line in Eq.~\refbra{eq:variance_weighted_clear}, an approximation, $\sum_j^{n}  \LSq x_{ij} w_i \RSq^2 \approx {x_i^\prime}^2$, is used since it is a usual case that values of weights satisfy $w_0 \sim 1>> w_1 >> w_2 >> \cdots >> w_n $ 
when a corresponding average of $\pThat$ is $ {\hat{p}_{T0}} < {\hat{p}_{T1}} < {\hat{p}_{T2}} < \cdots < {\hat{p}_{Tn}} $.
The meaning of Eq.~\refbra{eq:average_weighted_clear}, \refbra{eq:variance_weighted_clear}, and \refbra{eq:SE_weighted_clear} would be clear now. These are having forms of average, variance, and standard error for $N_\pThat$ events. 

Finally I mention some applicability of each definition of standard error.
As I already mentioned at the beginning of this section, one has to use these two different definitions depending on whether one generated event is considered as one complete event or not.
Besides that, notice that weights should be normalized if one uses Eq.~\refbra{eq:statval_weighted} while that is not necessary to be done for Eq.~\refbra{eq:statval_weighted_normal}.
