# Supplementary material for: Unified description of high-energy nuclear collisions based on dynamical core--corona picture
Source: arXiv:2208.07029 source file (2022-08-15)
Supplement: Supplementary file 5 [file appendix_numHydro.tex]

\thispagestyle{fancy}

\subsubsection{(3+1)-D relativistic hydrodynamics}

\begin{itemize}
    \item Reference: 
    \item Language: 
\end{itemize}

The code of (3+1)-D hydrodynamics used in this thesis is
built by Tachibana in Ref.~\cite{Tachibana:2014yai},
therefore I leave the detailed explanation for the reference. The (3+1)-D hydrodynamics is solved with the Piecewise Parabolic Method (PPM).
The PPM is a robust algorithm to solve the Riemann problem with shock waves. The first implementation to numerical simulations of relativistic heavy-ion collisions was done by Hirano in Ref.~\cite{Hirano:2000eu}.
